# Supplementary material for: Robust preconditioning for coupled Stokes-Darcy problems with the Darcy problem in primal form
Source: arXiv:2001.05529 source file (2020-01-15)
Supplement: Supplementary file 1 [file appendix.tex]

% temporary location for the appendix constructing Tgne in the case where Gamma is piecewise C^2 - not intended to be in the paper
\appendix

\section{Definition of $E_{\epsilon}$ for piecewise $C^2$ curves}
\label{app:c1ext}

Suppose $\Gamma \subset \reals^2$ is a piecewise $C^2$ curve, partitioned into finitely many $C^2$ segments $\Gamma_i$. We will construct the extension operator $E_{\epsilon}$ for $\Gamma$ discussed in the text. Let $\mathbf{P}_i$ be the point at which $\Gamma_i, \Gamma_{i+1}$ meet, and $\theta_i$ be the angle at which they meet. We may suppose that $\theta_i \neq \pi$, as in this case $\Gamma_i, \Gamma_{i+1}$ could be joined together to one segment.  Let $\mathbf{n}_{\Gamma}$ be the normal to $\Gamma$, which is continuous on each $\Gamma_i$. For each $\Gamma_i$, we define the \emph{normal $\epsilon$-envelope}

$$\Gamma^{\mathbf{n}}_{\epsilon, i} := \{y \in\reals \ \mbox{such that} \ y = x + s \cdot \mathbf{n}(x) \mbox{ for some}  \ x\in \Gamma, s < \epsilon \}$$

Informally, the normal $\epsilon-$envelope to $\Gamma_i$ is the set of points reachable from $\Gamma_i$ and taking steps of length less than $\epsilon$ in the direction of the normal. Recalling the $\epsilon$-thick envelope of $\Gamma$ defined earlier as
$$\Gamma_{i, \epsilon} = \{y \in\Omega_p \ \mbox{such that} \ |y-x| < \epsilon \mbox{ for some}  \ x\in \Gamma \}, $$
we see that it consists of the union of all $\Gamma^{\mathbf{n}}_{\epsilon, i}$ as well as the union of all $\epsilon$-balls centered at $\mathbf{P}_i$. Choosing $\epsilon$ sufficiently small, we see that the normal envelope is parametrized \keh{I'm not sure whether this requires additional assumptions on $\Gamma_i$, to be honest - it's not completely obvious, although it sounds true.}  by $\mathbf{x} \in \Gamma_i, s \in [0, \epsilon]$ as $\mathbf{g}_i(\mathbf{x}, s) := \mathbf{x} + t \cdot \mathbf{n}(\mathbf{x})$.

As illustrated in \cref{fig:c1segmentintersect}, this means that we can define $\mathbf{n}_{\Gamma_{\epsilon}}$ on all of $\Gamma_{\epsilon}$ by defining it on each $\Gamma^{\mathbf{n}}_{\epsilon, i}$ (the blue/red areas in \cref{fig:c1segmentintersect}), on each $\epsilon$-ball (the green area in the \cref{fig:c1segmentintersect}) and resolving the conflict on each of the areas where two normal envelopes intersect (the purple area in the \cref{fig:c1segmentintersect}). We remark that by choosing $\epsilon$ sufficiently small, we need not consider situations where the envelopes of three or more segments intersect.

\begin{figure}[H] 
  \begin{center}
      \includegraphics[width=0.49\linewidth]{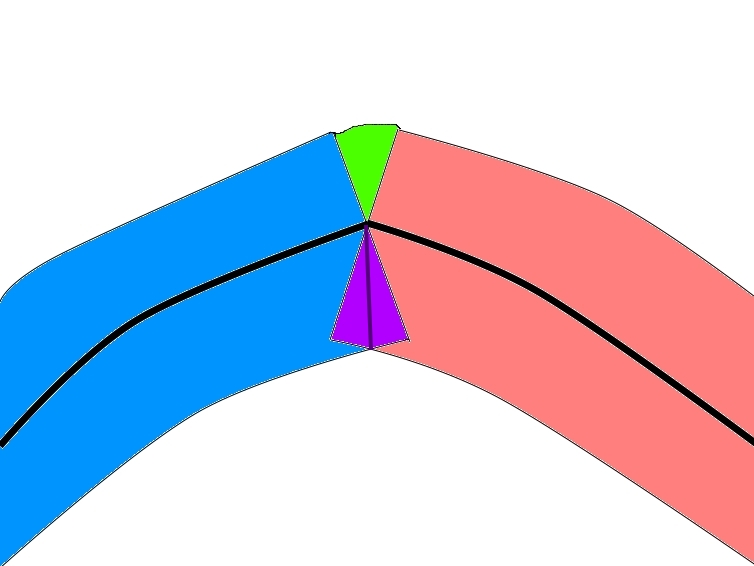} 
    \end{center}

    \caption{\textbf{Placeholder} illustration of what happens at $\mathbf{P}_i$ where $\Gamma_i$ and $\Gamma_{i+i}$ intersect. The blue area is the normal $\epsilon$-envelope of $\Gamma_i$, and the red area is the normal $\epsilon$-envelope of $\Gamma_{i+1}$. The green area is a circle sector of angle $\frac {\pi - \theta_i} 2$ and radius $\epsilon$, and is contained in the $\epsilon$-envelope of $\Gamma$, but none of the normal $\epsilon$-envelopes of any $\Gamma_j$, while the purple area is contained in both normal $\epsilon$-envelopes. The dark purple line is the angular bisector of $\theta_i$. \label{fig:c1segmentintersect}
    }
    \vspace{5pt}    
\end{figure}

As $\Gamma_i$ is $C^2$, it has a normal vector $\mathbf{n}(\mathbf{x})$ for any $\mathbf{x} \in \Gamma_i$. Hence we can define an extension $\mathbf{n}^{\epsilon}_{\Gamma_i}$ on all of $\Gamma^{\mathbf{n}}_{\epsilon, i}$ by sending a point $\mathbf{g}_i(\mathbf{x}, s)$ to $\mathbf{n}(\mathbf{x})$. Each intersection $\Gamma^{\mathbf{n}}_{\epsilon, i} \cap \Gamma^{\mathbf{n}}_{\epsilon, i+1}$ is split in two by the angular bisector of $\theta_i$, and on this intersection we define $\mathbf{n}_{\Gamma_{\epsilon}}$ to be the extension $\mathbf{n}^{\epsilon}_{\Gamma_i}$ on the half closest to $\Gamma_i$, and $\mathbf{n}^{\epsilon}_{\Gamma_{i+1}}$ on the other half.

This defines $\mathbf{n}_{\Gamma_{\epsilon}}$ on all points which are in the normal envelope of some segment. All other points of $\Gamma_{\epsilon}$ are in the areas marked green in \cref{fig:c1segmentintersect}. Each such area is a circle sector centered at a $\mathbf{P}_i$, and is of radius $\epsilon$ and angle $\psi_i := \frac {\pi - \theta_i} 2$. Parametrizing this sector by polar coordinates centered at $\mathbf{P}_i$, we define $\mathbf{n}_{\Gamma_{\epsilon}}$ to be the unit radial vector in these coordinates, so that it matches $\mathbf{n}^{\epsilon}_{\Gamma_{i}}$ on the left edge, and $\mathbf{n}^{\epsilon}_{\Gamma_{i+1}}$ on the right edge.

This defines $\mathbf{n}_{\epsilon}$ on all parts of $\Gamma_{\epsilon}$. Per construction, it is piecewise continuous, with discontinuities exactly where the blue and red areas meet the purple area in \cref{fig:c1segmentintersect}. Next, we define the required extension $E_{\epsilon} : L^2(\Gamma) \to L^2(\Gamma_{\epsilon})$. Given any smooth $w \in C^{\infty}(\Gamma)$, we define $E_{\epsilon}w$ in the same piecewise manner. If a point $\mathbf{y} \in \Gamma_{\epsilon}$ is in the (red or blue) normal envelope of exactly one segment $\Gamma_i$, we use the parametrization $\mathbf{g}_i$ from above to find unique $\mathbf{x}, t$ so that $\mathbf{y} = \mathbf{x} + t \cdot \mathbf{n}(\mathbf{x})$ and define $\left ( E_{\epsilon}w \right) (\mathbf{y}) := w (\mathbf{x})$.

If $\mathbf{y}$ is in the (purple) intersection of two envelopes $\Gamma^{\mathbf{n}}_{\epsilon, i} \cap \Gamma^{\mathbf{n}}_{\epsilon, i+1}$, we divide the intersection in two by the angular bisector of $\theta_i$, and use the definition of $E_{\epsilon}w$ from $\Gamma_i$ if $\mathbf{y}$ is on the side closest to $\Gamma_i$, and otherwise the definition from $\Gamma_{i+1}$. Finally, all other $\mathbf{y}\in \Gamma_{\epsilon}$ not of any of the two previous forms are in some (green) $\mathbf{\epsilon}$-ball around a $\mathbf{P}_i$, and for such $\mathbf{y}$ we define $\left ( E_{\epsilon}w \right) (\mathbf{y}) := w(\mathbf{P}_i)$. This defines $E_{\epsilon}w$ uniquely for a smooth $w$. By continuity, we may then extend to an operator $E_{\epsilon}: L^2(\Gamma) \to L^2(\Gamma_{\epsilon})$, yielding the required extension.
